# Supplementary material for: Recent Developments and Perspectives in Variational Quantum Eigensolvers for Molecular Electronic Structure: Methods, Tradeoffs, and Benchmarking
Source: arXiv:2602.11384 source file (2026-07-17)
Supplement: Supplementary file 1 [file VQE_Survey_Supporting_Information.pdf]

# Recent Developments in VQE: Survey and Benchmarking

Taylor Harville, Rishu Khurana, Vitor F. Grizzi, Cong Liu\*

Chemical Sciences and Engineering Division, Argonne National Laboratory, Lemont, IL, 60439,  
United States  
E-mail: congliu@anl.gov

## Computational Details:

All fully classical calculations (RHF, CCSD(T), UCCSD(T), and FCI) were performed with either the STO-3G or 6-31G basis sets using the PySCF<sup>1-3</sup> software package. ADAPT-VQE and USCC were both installed using the recommended packages published alongside the code repositories on GitHub linked in the original publication including use of the published environments.yml and requirements.txt files listing all software dependencies.

**Number of parameters for each calculation for VQE, ADAPT-VQE, and USCC at each threshold value for each radius:**

| H <sub>6</sub> //STO-3G | VQE | ADAPT-VQE |     |     |     | USCC E-1 |     |     |     |
|-------------------------|-----|-----------|-----|-----|-----|----------|-----|-----|-----|
| R (Angstrom)            |     | E-1       | E-2 | E-3 | E-4 | E-1      | E-2 | E-3 | E-4 |
| 0.50                    | 3   | 1         | 1   | 1   | 1   | 0        | 1   | 1   | 1   |
| 0.77                    | 3   | 1         | 1   | 1   | 1   | 0        | 1   | 1   | 1   |
| 1.04                    | 3   | 1         | 1   | 1   | 1   | 0        | 1   | 1   | 1   |
| 1.31                    | 3   | 1         | 1   | 1   | 1   | 1        | 1   | 1   | 1   |
| 1.58                    | 3   | 1         | 1   | 1   | 1   | 1        | 1   | 1   | 1   |
| 1.85                    | 3   | 1         | 1   | 1   | 1   | 1        | 1   | 1   | 1   |
| 2.12                    | 3   | 1         | 1   | 1   | 1   | 1        | 1   | 1   | 1   |
| 2.38                    | 3   | 1         | 1   | 1   | 1   | 1        | 1   | 1   | 1   |
| 2.65                    | 3   | 1         | 1   | 1   | 1   | 1        | 1   | 1   | 1   |
| 2.92                    | 3   | 1         | 1   | 1   | 1   | 1        | 1   | 1   | 1   |
| 3.19                    | 3   | 1         | 1   | 1   | 1   | 1        | 1   | 1   | 1   |
| 3.46                    | 3   | 1         | 1   | 1   | 1   | 1        | 1   | 1   | 1   |
| 3.73                    | 3   | 1         | 1   | 1   | 1   | 1        | 1   | 1   | 1   |
| 4.00                    | 3   | 1         | 1   | 1   | 1   | 1        | 1   | 1   | 1   |

| LiH//STO-3G  | VQE | ADAPT-VQE |     |     |     | USCC |     |     |     |
|--------------|-----|-----------|-----|-----|-----|------|-----|-----|-----|
| R (Angstrom) |     | E-1       | E-2 | E-3 | E-4 | E-1  | E-2 | E-3 | E-4 |
| 0.8          | 92  | 2         | 16  | 21  | 25  | 6    | 18  | 48  | 68  |
| 1.05         | 92  | 2         | 15  | 21  | 25  | 4    | 13  | 46  | 68  |
| 1.29         | 92  | 1         | 15  | 21  | 24  | 4    | 12  | 41  | 68  |
| 1.54         | 92  | 1         | 13  | 22  | 26  | 2    | 14  | 33  | 68  |
| 1.78         | 92  | 2         | 14  | 23  | 25  | 2    | 12  | 45  | 68  |
| 2.03         | 92  | 2         | 14  | 22  | 25  | 2    | 14  | 45  | 68  |
| 2.28         | 92  | 2         | 15  | 22  | 25  | 2    | 13  | 39  | 67  |
| 2.52         | 92  | 2         | 16  | 23  | 25  | 2    | 13  | 43  | 67  |
| 2.77         | 92  | 3         | 16  | 23  | 25  | 2    | 15  | 49  | 67  |
| 3.02         | 92  | 3         | 18  | 23  | 25  | 2    | 15  | 49  | 67  |
| 3.26         | 92  | 4         | 19  | 24  | 25  | 2    | 15  | 47  | 67  |
| 3.51         | 92  | 4         | 19  | 25  | 25  | 2    | 15  | 43  | 67  |
| 3.75         | 92  | 4         | 19  | 25  | 25  | 2    | 14  | 43  | 67  |
| 4            | 92  | 4         | 18  | 24  | 25  | 2    | 12  | 39  | 67  |

| H <sub>2</sub> O//STO-3G | VQE | ADAPT-VQE |     |     |     | USCC |     |     |     |
|--------------------------|-----|-----------|-----|-----|-----|------|-----|-----|-----|
| R (Angstrom)             |     | E-1       | E-2 | E-3 | E-4 | E-1  | E-2 | E-3 | E-4 |
| 0.50                     | 140 | 10        | 23  | 30  | 53  | 8    | 27  | 94  | 144 |
| 0.71                     | 140 | 11        | 24  | 42  | 62  | 8    | 36  | 107 | 212 |
| 0.91                     | 140 | 12        | 27  | 44  | 66  | 8    | 38  | 133 | 220 |
| 1.12                     | 140 | 13        | 27  | 49  | 75  | 8    | 37  | 138 | 228 |
| 1.33                     | 140 | 11        | 32  | 58  | 82  | 8    | 35  | 137 | 218 |
| 1.53                     | 140 | 11        | 30  | 54  | 81  | 8    | 32  | 135 | 218 |
| 1.74                     | 140 | 12        | 26  | 59  | 87  | 6    | 34  | 151 | 218 |
| 1.95                     | 140 | 10        | 32  | 63  | 89  | 11   | 56  | 153 | 227 |
| 2.16                     | 140 | 6         | 23  | 61  | 94  | 8    | 45  | 125 | 190 |
| 2.50                     | 140 | 4         | 9   | 40  | 61  | 5    | 22  | 57  | 115 |

| H <sub>6</sub> //STO-3G | VQE | ADAPT-VQE |     |     |     | USCC |     |     |     |
|-------------------------|-----|-----------|-----|-----|-----|------|-----|-----|-----|
| R (Angstrom)            |     | E-1       | E-2 | E-3 | E-4 | E-1  | E-2 | E-3 | E-4 |
| 0.50                    | 117 | 24        | 48  | 61  | 95  | 4    | 57  | 199 | 364 |
| 0.71                    | 117 | 25        | 49  | 73  | 105 | 4    | 57  | 226 | 374 |
| 0.91                    | 117 | 25        | 51  | 86  | 113 | 4    | 61  | 264 | 380 |
| 1.12                    | 117 | 25        | 57  | 96  | 126 | 4    | 65  | 292 | 380 |
| 1.33                    | 117 | 25        | 61  | 106 | 145 | 4    | 65  | 320 | 380 |
| 1.53                    | 117 | 25        | 72  | 122 | 153 | 4    | 75  | 350 | 380 |
| 1.74                    | 117 | 25        | 76  | 129 | 161 | 2    | 73  | 378 | 380 |
| 1.95                    | 117 | 19        | 76  | 141 | 164 | 2    | 83  | 380 | 380 |
| 2.16                    | 117 | 9         | 80  | 151 | 169 | 0    | 93  | 380 | 380 |
| 2.50                    | 117 | 9         | 34  | 156 | 174 | 0    | 99  | 378 | 380 |

| BeH <sub>2</sub> //STO-3G | VQE | ADAPT-VQE |     |     |     | USCC |     |     |     |
|---------------------------|-----|-----------|-----|-----|-----|------|-----|-----|-----|
| R (Angstrom)              |     | E-1       | E-2 | E-3 | E-4 | E-1  | E-2 | E-3 | E-4 |
| 0.50                      | 204 | 15        | 40  | 54  | 70  | 12   | 42  | 170 | 269 |
| 0.76                      | 204 | 9         | 35  | 34  | 65  | 6    | 24  | 109 | 225 |
| 1.02                      | 204 | 9         | 35  | 46  | 66  | 4    | 31  | 107 | 244 |
| 1.28                      | 204 | 9         | 33  | 48  | 69  | 4    | 28  | 99  | 247 |
| 1.53                      | 204 | 10        | 32  | 50  | 78  | 8    | 29  | 106 | 261 |
| 1.79                      | 204 | 10        | 36  | 53  | 74  | 10   | 31  | 122 | 275 |
| 2.05                      | 204 | 11        | 37  | 57  | 86  | 10   | 31  | 124 | 275 |
| 2.31                      | 204 | 11        | 38  | 69  | 86  | 10   | 31  | 141 | 275 |
| 2.57                      | 204 | 11        | 39  | 63  | 79  | 10   | 30  | 143 | 277 |
| 2.74                      | 204 | 11        | 36  | 64  | 81  | 8    | 30  | 147 | 273 |
| 3.00                      | 204 | 12        | 35  | 59  | 76  | 8    | 24  | 147 | 269 |

Citations:

1. Recent developments in the PySCF program package, Q. Sun, X. Zhang, S. Banerjee, P. Bao, M. Barbry, N. S. Blunt, N. A. Bogdanov, G. H. Booth, J. Chen, Z.-H. Cui, J. J. Eriksen, Y. Gao, S. Guo, J. Hermann, M. R. Hermes, K. Koh, P. Koval, S. Lehtola, Z. Li, J. Liu, N. Mardirossian, J. D. McClain, M. Motta, B. Mussard, H. Q. Pham, A. Pulkin, W. Purwanto, P. J. Robinson, E. Ronca, E. R. Sayfutyarova, M. Scheurer, H. F. Schurkus, J. E. T. Smith, C. Sun, S.-N. Sun, S. Upadhyay, L. K. Wagner, X. Wang, A. White, J. Daniel Whitfield, M. J. Williamson, S. Wouters, J. Yang, J. M. Yu, T. Zhu, T. C. Berkelbach, S. Sharma, A. Yu. Sokolov, and G. K.-L. Chan, *J. Chem. Phys.* 153, 024109 (2020)
2. PySCF: the Python-based simulations of chemistry framework, Q. Sun, T. C. Berkelbach, N. S. Blunt, G. H. Booth, S. Guo, Z. Li, J. Liu, J. McClain, S. Sharma, S. Wouters, and G. K.-L. Chan, *WIREs Comput. Mol. Sci.* 8, e1340 (2018)
3. Libcint: An efficient general integral library for Gaussian basis functions, Q. Sun, J. *Comp. Chem.* 36, 1664 (2015)
